# Supplementary material for: Flow-Induced Diagonal Gaussian Processes
Source: arXiv:2509.17153 source file (2025-10-02)
Supplement: Supplementary file 1 [file 7-appendix.tex]

\appendix
\subsection{Appendix A: Proof of Spectral Residual Separation}

\textbf{Lemma (Spectral Residual Separation)}  
Let the weight matrix be decomposed as
\begin{equation}
w = T_{\mathrm{row}} U T_{\mathrm{col}}^\top + E
\end{equation}
where $T_{\mathrm{row}} \in \mathbb{R}^{n \times r}$, $U \in \mathbb{R}^{r \times r}$, $T_{\mathrm{col}} \in \mathbb{R}^{d \times r}$. Define the separation margin and residual as:
\begin{equation}
S = \inf_{\|x\|=1}\left\|(I - P)\, g(T_{\mathrm{row}} U T_{\mathrm{col}}^\top x)\right\|
\end{equation}
\begin{equation}
d(x) = \left\|(I - P)\, g((T_{\mathrm{row}} U T_{\mathrm{col}}^\top + E)x)\right\|
\end{equation}
with projection $P$ given by
\begin{equation}
P = U^\top (U U^\top + \lambda I)^{-1} U
\end{equation}
satisfying $\|I - P\|_\sigma = 1$. The mapping $g:\mathbb{R}^n \to \mathbb{R}^{r \times r}$ is 1-Lipschitz under Frobenius norm.

For in-distribution (ID) samples, we enforce via loss function:
\begin{equation}
L_{\mathrm{ID}} = \left\|(I - P)\, g(T_{\mathrm{row}} U T_{\mathrm{col}}^\top x_{\mathrm{ID}})\right\|_2 = 0
\end{equation}
thus
\begin{equation}
(I - P)\, g(T_{\mathrm{row}} U T_{\mathrm{col}}^\top x_{\mathrm{ID}}) = 0
\end{equation}
and empirically observe:
\begin{equation}
\sup_{x_{\mathrm{ID}}} d(x_{\mathrm{ID}}) < \|E\|
\end{equation}

If during training we achieve (empirically) for out-of-distribution (OoD) samples:
\begin{equation}
S_{\mathrm{OoD}} > 2\,\|E\|
\end{equation}
then strict separation holds:
\begin{equation}
\sup_{x_{\mathrm{ID}}} d\bigl(x_{\mathrm{ID}}\bigr)
\;<\;
\inf_{x_{\mathrm{OoD}}} d\bigl(x_{\mathrm{OoD}}\bigr)
\end{equation}

\medskip
\noindent\textbf{Proof.}  
Assume $\|x\| = 1$ for all samples. We establish bounds:

\medskip
\noindent\textbf{Step 1: ID residual bound.}  
For any $x_{\mathrm{ID}}$:
\begin{equation}
\begin{aligned}
d(x_{\mathrm{ID}}) 
&= \left\|(I - P)\left[g(w x_{\mathrm{ID}}) - g(T_{\mathrm{row}} U T_{\mathrm{col}}^\top x_{\mathrm{ID}})\right]\right\| \\
&\leq \|I - P\|_\sigma \left\|g(w x_{\mathrm{ID}}) - g(T_{\mathrm{row}} U T_{\mathrm{col}}^\top x_{\mathrm{ID}})\right\| \\
&\leq \|E x_{\mathrm{ID}}\|_F \quad \text{($g$ 1-Lipschitz)} \\
&\leq \|E\| \|x_{\mathrm{ID}}\| = \|E\|
\end{aligned}
\end{equation}
Thus:
\begin{equation}
\sup_{x_{\mathrm{ID}}} d(x_{\mathrm{ID}}) \leq \|E\|
\end{equation}

\medskip
\noindent\textbf{Step 2: OoD residual bound.}  
For any $x_{\mathrm{OoD}}$:
\begin{equation}
\begin{aligned}
d(x_{\mathrm{OoD}}) 
&\geq \left| \left\|(I - P) g(T_{\mathrm{row}} U T_{\mathrm{col}}^\top x_{\mathrm{OoD}})\right\| \right. \\
&\quad - \left. \left\|(I - P)\left[g(w x_{\mathrm{OoD}}) - g(T_{\mathrm{row}} U T_{\mathrm{col}}^\top x_{\mathrm{OoD}})\right]\right\| \right| \\
&\geq S_{\mathrm{OoD}} - \|I - P\|_\sigma \|E x_{\mathrm{OoD}}\|_F \\
&\geq S_{\mathrm{OoD}} - \|E\|
\end{aligned}
\end{equation}
Therefore:
\begin{equation}
\inf_{x_{\mathrm{OoD}}} d(x_{\mathrm{OoD}}) \geq S_{\mathrm{OoD}} - \|E\|
\end{equation}

\medskip
\noindent\textbf{Step 3: Strict separation.}  
Given $S_{\mathrm{OoD}} > 2\|E\|$:
\begin{equation}
\begin{aligned}
\sup_{x_{\mathrm{ID}}} d(x_{\mathrm{ID}}) 
&\leq \|E\| \\
&< S_{\mathrm{OoD}} - \|E\| \\
&\leq \inf_{x_{\mathrm{OoD}}} d(x_{\mathrm{OoD}})
\end{aligned}
\end{equation}
which completes the proof. \qed
